# Supplementary material for: A Machine Learning Early Warning System: Multicenter Validation in Brazilian Hospitals
Source: arXiv:2006.05514 source file (2020-06-09)
Supplement: Supplementary file 1 [file supp.tex]

%%% Supplementary Material

\\
\begin{table}[] \centering
\caption{Leave One Hospital Out.}
\label{tab:LOHO}
\begin{tabular}{llllllll}
 & \multicolumn{7}{c}{XGBoost} \\
 & H1 & H2 & H3 & H4 & H5 & H6 & mean \\
specificity & 0.960270 & 0.989260 & 0.829073 & 0.974317 & 0.917323 & 0.928797 & 0.933173 \\
recall & 0.892958 & 0.539349 & 0.746136 & 0.811951 & 0.962617 & 0.833554 & 0.797761 \\
precision & 0.366474 & 0.674541 & 0.380188 & 0.522034 & 0.412000 & 0.363689 & 0.453154 \\
f1 & 0.519672 & 0.599417 & 0.503713 & 0.635488 & 0.577031 & 0.506421 & 0.556957 \\
mcc & 0.556996 & 0.588729 & 0.441541 & 0.636593 & 0.600319 & 0.520237 & 0.557402 \\
auc & 0.982198 & 0.929673 & 0.875561 & 0.956708 & 0.988336 & 0.952533 & 0.947502 \\
 &  &  &  &  &  &  &  \\
 & \multicolumn{7}{c}{LightBoost} \\
 & H1 & H2 & H3 & H4 & H5 & H6 & mean \\
specificity & 0.929167 & 0.980166 & 0.735923 & 0.960959 & 0.847019 & 0.876782 & 0.888336 \\
recall & 0.946479 & 0.606506 & 0.837693 & 0.857645 & 0.971963 & 0.892338 & 0.852104 \\
precision & 0.255903 & 0.557915 & 0.308315 & 0.431477 & 0.276596 & 0.261214 & 0.348570 \\
f1 & 0.402878 & 0.581197 & 0.450736 & 0.574118 & 0.430642 & 0.404128 & 0.473950 \\
mcc & 0.472000 & 0.563695 & 0.399515 & 0.590796 & 0.474235 & 0.443082 & 0.490554 \\
auc & 0.985196 & 0.930721 & 0.879299 & 0.957988 & 0.986554 & 0.952274 & 0.948672 \\
 &  &  &  &  &  &  &  \\
 & \multicolumn{7}{c}{CatBoost} \\
 & H1 & H2 & H3 & H4 & H5 & H6 & mean \\
specificity & 0.381425 & 0.494024 & 0.194737 & 0.538373 & 0.167042 & 0.296356 & 0.345326 \\
recall & 0.997183 & 0.965373 & 0.972057 & 0.961336 & 1.000.000 & 0.981506 & 0.979576 \\
precision & 0.039838 & 0.072993 & 0.145024 & 0.067117 & 0.067380 & 0.063760 & 0.076019 \\
f1 & 0.076615 & 0.135723 & 0.252393 & 0.125473 & 0.126254 & 0.119742 & 0.139367 \\
mcc & 0.122520 & 0.179465 & 0.144542 & 0.179727 & 0.106091 & 0.129894 & 0.143707 \\
auc & 0.971964 & 0.920856 & 0.845570 & 0.948071 & 0.977332 & 0.930655 & 0.932408 \\
 &  &  &  &  &  &  &  \\
 & \multicolumn{7}{c}{Logistic Regression} \\
 & H1 & H2 & H3 & H4 & H5 & H6 & mean \\
specificity & 0.857536 & 0.933440 & 0.664912 & 0.922344 & 0.804274 & 0.875298 & 0.842968 \\
recall & 0.963380 & 0.684155 & 0.839477 & 0.852373 & 0.971963 & 0.863276 & 0.862437 \\
precision & 0.148244 & 0.297853 & 0.260372 & 0.274943 & 0.230088 & 0.252609 & 0.244018 \\
f1 & 0.256950 & 0.415022 & 0.397467 & 0.415774 & 0.372093 & 0.390849 & 0.374692 \\
mcc & 0.347556 & 0.418864 & 0.338791 & 0.456884 & 0.420688 & 0.425418 & 0.401367 \\
auc & 0.973362 & 0.918923 & 0.846011 & 0.937473 & 0.977692 & 0.938971 & 0.932072 \\
 &  &  &  &  &  &  &  \\
 & \multicolumn{7}{c}{Naive Bayes} \\
 & H1 & H2 & H3 & H4 & H5 & H6 & mean \\
specificity & 0.919959 & 0.953577 & 0.900835 & 0.946630 & 0.770529 & 0.746179 & 0.872952 \\
recall & 0.864789 & 0.438615 & 0.444114 & 0.771529 & 0.925234 & 0.760238 & 0.700753 \\
precision & 0.217576 & 0.280537 & 0.386246 & 0.333080 & 0.195266 & 0.127577 & 0.256714 \\
f1 & 0.347678 & 0.342202 & 0.413164 & 0.465289 & 0.322476 & 0.218489 & 0.351550 \\
mcc & 0.409616 & 0.317367 & 0.325133 & 0.482976 & 0.363070 & 0.238297 & 0.356076 \\
auc & 0.952623 & 0.830540 & 0.645930 & 0.928274 & 0.926406 & 0.836826 & 0.853433 \\
 &  &  &  &  &  &  &  \\
 & \multicolumn{7}{c}{Random Forest} \\
 & H1 & H2 & H3 & H4 & H5 & H6 & mean \\
specificity & 0.843761 & 0.931665 & 0.601086 & 0.902125 & 0.709224 & 0.663012 & 0.775145 \\
recall & 0.963380 & 0.693599 & 0.885850 & 0.901582 & 1.000.000 & 0.943857 & 0.898045 \\
precision & 0.136964 & 0.295221 & 0.237829 & 0.241412 & 0.171474 & 0.120296 & 0.200533 \\
f1 & 0.239832 & 0.414160 & 0.374984 & 0.380846 & 0.292750 & 0.213395 & 0.319328 \\
mcc & 0.331133 & 0.419784 & 0.321172 & 0.437043 & 0.348732 & 0.265529 & 0.353899 \\
auc & 0.980774 & 0.883220 & 0.860105 & 0.945402 & 0.985816 & 0.942551 & 0.932978
\end{tabular}
\end{table}

Entity ID: all, Count 121522
MODEL   AUC     F1      TIME
XGBoost	 0.9559 (0.632) 10.02 s
LogReg	 0.9326 (0.5565) 967.61 s
D.Tree	 0.7482 (0.4994) 156.02 s
RForest	 0.9406 (0.609) 546.14 s
CatBoos	 0.9555 (0.6426) 31.79 s
Naive	 0.8418 (0.3793) 3.45 s
Light	 0.9611 (0.6715) 312.0 s

Número de Colunas: 11 Exame(s): 1
['document.glicemia_capilar(t-4)', 'document.pa_diastolica(t-4)', 'UTI', 'age', 'document.sexo', 'document.temperatura(t-4)', 'document.freq_cardiaca(t-4)', 'document.freq_respiratoria(t-4)', 'document.pa_sistolica(t-4)', 'days_from_entrance', 'document.sat_o2(t-4)']
	XGBoost	 0.9285 (+-0.0047) 2.96 s
	LogReg	 0.9047 (+-0.0054) 11.25 s
	D.Tree	 0.7107 (+-0.0074) 7.48 s
	RForest	 0.9064 (+-0.0046) 72.15 s
	CatBoos	 0.9301 (+-0.0045) 9.83 s
	Naive	 0.8578 (+-0.006) 0.44 s
	Light	 0.9354 (+-0.0044) 44.18 s
Número de Colunas: 25 Exame(s): 2
['delta_document.pa_sistolica_t3-t4', 'document.freq_cardiaca(t-4)', 'document.sat_o2(t-4)', 'document.pa_sistolica(t-3)', 'document.sat_o2(t-3)', 'delta_document.temperatura_t3-t4', 'document.glicemia_capilar(t-4)', 'document.freq_respiratoria(t-3)', 'UTI', 'age', 'document.sexo', 'days_from_entrance', 'document.freq_cardiaca(t-3)', 'delta_document.pa_diastolica_t3-t4', 'delta_document.sat_o2_t3-t4', 'delta_document.freq_respiratoria_t3-t4', 'document.temperatura(t-4)', 'document.pa_diastolica(t-3)', 'document.glicemia_capilar(t-3)', 'document.pa_sistolica(t-4)', 'document.pa_diastolica(t-4)', 'delta_document.glicemia_capilar_t3-t4', 'document.freq_respiratoria(t-4)', 'document.temperatura(t-3)', 'delta_document.freq_cardiaca_t3-t4']
	XGBoost	 0.9374 (+-0.005) 4.18 s
	LogReg	 0.9138 (+-0.0064) 43.98 s
	D.Tree	 0.7192 (+-0.0116) 20.04 s
	RForest	 0.9141 (+-0.0085) 130.24 s
	CatBoos	 0.9379 (+-0.0049) 13.25 s
	Naive	 0.8337 (+-0.0067) 0.67 s
	Light	 0.943 (+-0.0042) 71.26 s
Número de Colunas: 39 Exame(s): 3
['delta_document.pa_sistolica_t3-t4', 'delta_document.pa_diastolica_t2-t3', 'document.freq_cardiaca(t-4)', 'document.sat_o2(t-4)', 'document.pa_sistolica(t-3)', 'document.sat_o2(t-3)', 'delta_document.temperatura_t3-t4', 'document.glicemia_capilar(t-4)', 'document.freq_respiratoria(t-3)', 'delta_document.sat_o2_t2-t3', 'UTI', 'age', 'document.sexo', 'document.pa_diastolica(t-2)', 'delta_document.temperatura_t2-t3', 'document.sat_o2(t-2)', 'days_from_entrance', 'delta_document.sat_o2_t3-t4', 'delta_document.pa_diastolica_t3-t4', 'document.freq_cardiaca(t-3)', 'delta_document.freq_respiratoria_t3-t4', 'document.freq_cardiaca(t-2)', 'delta_document.pa_sistolica_t2-t3', 'document.temperatura(t-4)', 'delta_document.freq_cardiaca_t2-t3', 'document.pa_diastolica(t-3)', 'document.glicemia_capilar(t-3)', 'document.pa_sistolica(t-4)', 'document.pa_sistolica(t-2)', 'document.pa_diastolica(t-4)', 'delta_document.glicemia_capilar_t3-t4', 'document.glicemia_capilar(t-2)', 'document.freq_respiratoria(t-2)', 'document.freq_respiratoria(t-4)', 'document.temperatura(t-3)', 'delta_document.freq_cardiaca_t3-t4', 'document.temperatura(t-2)', 'delta_document.freq_respiratoria_t2-t3', 'delta_document.glicemia_capilar_t2-t3']
	XGBoost	 0.944 (+-0.0045) 4.35 s
	LogReg	 0.9201 (+-0.0058) 122.47 s
	D.Tree	 0.7272 (+-0.0084) 35.78 s
	RForest	 0.9237 (+-0.0074) 174.16 s
	CatBoos	 0.9445 (+-0.0046) 14.22 s
	Naive	 0.8316 (+-0.0074) 1.08 s
	Light	 0.9495 (+-0.0041) 100.16 s
Número de Colunas: 53 Exame(s): 4
['delta_document.pa_diastolica_t2-t3', 'delta_document.pa_sistolica_t3-t4', 'document.freq_cardiaca(t-4)', 'document.freq_respiratoria(t-1)', 'document.glicemia_capilar(t-1)', 'document.sat_o2(t-4)', 'document.pa_sistolica(t-3)', 'document.sat_o2(t-3)', 'delta_document.temperatura_t3-t4', 'delta_document.pa_diastolica_t1-t2', 'document.glicemia_capilar(t-4)', 'document.freq_respiratoria(t-3)', 'delta_document.sat_o2_t2-t3', 'document.pa_sistolica(t-1)', 'UTI', 'age', 'document.sexo', 'document.freq_cardiaca(t-1)', 'document.pa_diastolica(t-2)', 'delta_document.temperatura_t2-t3', 'document.sat_o2(t-2)', 'days_from_entrance', 'delta_document.sat_o2_t3-t4', 'delta_document.pa_diastolica_t3-t4', 'document.freq_cardiaca(t-3)', 'delta_document.glicemia_capilar_t1-t2', 'delta_document.freq_respiratoria_t3-t4', 'document.freq_cardiaca(t-2)', 'delta_document.pa_sistolica_t2-t3', 'document.sat_o2(t-1)', 'document.temperatura(t-4)', 'delta_document.freq_cardiaca_t2-t3', 'document.temperatura(t-1)', 'document.pa_diastolica(t-3)', 'delta_document.freq_cardiaca_t1-t2', 'document.glicemia_capilar(t-3)', 'document.pa_sistolica(t-4)', 'document.pa_diastolica(t-1)', 'delta_document.sat_o2_t1-t2', 'document.pa_sistolica(t-2)', 'document.pa_diastolica(t-4)', 'delta_document.glicemia_capilar_t3-t4', 'delta_document.pa_sistolica_t1-t2', 'delta_document.temperatura_t1-t2', 'document.glicemia_capilar(t-2)', 'document.freq_respiratoria(t-2)', 'document.freq_respiratoria(t-4)', 'document.temperatura(t-3)', 'delta_document.freq_cardiaca_t3-t4', 'document.temperatura(t-2)', 'delta_document.freq_respiratoria_t2-t3', 'delta_document.glicemia_capilar_t2-t3', 'delta_document.freq_respiratoria_t1-t2']
	XGBoost	 0.9506 (+-0.0043) 5.3 s
	LogReg	 0.9286 (+-0.005) 236.43 s
	D.Tree	 0.7362 (+-0.0049) 58.34 s
	RForest	 0.9327 (+-0.0055) 221.28 s
	CatBoos	 0.9502 (+-0.0041) 15.24 s
	Naive	 0.8366 (+-0.007) 1.51 s
	Light	 0.9559 (+-0.0038) 128.46 s
Número de Colunas: 67 Exame(s): 5
['delta_document.pa_diastolica_t2-t3', 'delta_document.pa_sistolica_t3-t4', 'document.freq_cardiaca(t-4)', 'document.glicemia_capilar(t-1)', 'document.freq_respiratoria(t-1)', 'delta_document.pa_sistolica_t-t1', 'document.sat_o2(t-4)', 'document.pa_sistolica(t)', 'document.pa_sistolica(t-3)', 'document.sat_o2(t-3)', 'delta_document.temperatura_t3-t4', 'delta_document.pa_diastolica_t1-t2', 'document.glicemia_capilar(t-4)', 'document.freq_respiratoria(t-3)', 'delta_document.sat_o2_t2-t3', 'document.freq_cardiaca(t)', 'document.pa_sistolica(t-1)', 'document.pa_diastolica(t)', 'UTI', 'age', 'document.sexo', 'document.freq_cardiaca(t-1)', 'delta_document.temperatura_t-t1', 'document.pa_diastolica(t-2)', 'delta_document.temperatura_t2-t3', 'document.sat_o2(t-2)', 'days_from_entrance', 'delta_document.glicemia_capilar_t-t1', 'delta_document.sat_o2_t3-t4', 'delta_document.pa_diastolica_t3-t4', 'document.freq_cardiaca(t-3)', 'document.freq_respiratoria(t)', 'delta_document.glicemia_capilar_t1-t2', 'delta_document.freq_respiratoria_t3-t4', 'document.freq_cardiaca(t-2)', 'delta_document.pa_sistolica_t2-t3', 'delta_document.freq_cardiaca_t-t1', 'document.temperatura(t-4)', 'document.temperatura(t)', 'delta_document.freq_cardiaca_t2-t3', 'document.temperatura(t-1)', 'document.pa_diastolica(t-3)', 'delta_document.freq_cardiaca_t1-t2', 'document.glicemia_capilar(t-3)', 'delta_document.pa_diastolica_t-t1', 'document.pa_sistolica(t-4)', 'document.pa_diastolica(t-1)', 'document.glicemia_capilar(t)', 'delta_document.sat_o2_t1-t2', 'document.pa_sistolica(t-2)', 'delta_document.freq_respiratoria_t-t1', 'delta_document.sat_o2_t-t1', 'document.pa_diastolica(t-4)', 'delta_document.freq_respiratoria_t2-t3', 'document.sat_o2(t)', 'delta_document.glicemia_capilar_t3-t4', 'delta_document.pa_sistolica_t1-t2', 'delta_document.temperatura_t1-t2', 'document.glicemia_capilar(t-2)', 'document.freq_respiratoria(t-2)', 'document.freq_respiratoria(t-4)', 'document.temperatura(t-3)', 'delta_document.freq_cardiaca_t3-t4', 'document.temperatura(t-2)', 'document.sat_o2(t-1)', 'delta_document.glicemia_capilar_t2-t3', 'delta_document.freq_respiratoria_t1-t2']
	XGBoost	 0.9559 (+-0.0039) 5.1 s
	LogReg	 0.9326 (+-0.0055) 493.28 s
	D.Tree	 0.7465 (+-0.0076) 78.28 s
	RForest	 0.9402 (+-0.006) 271.72 s
	CatBoos	 0.9555 (+-0.0041) 15.67 s
	Naive	 0.8418 (+-0.0068) 1.76 s
	Light	 0.9611 (+-0.0039) 156.87 s
	
MEWS, AUC, F1

---- t4 -----
0 0.5042 0.0965
1 0.6584 0.1634
2 0.626 0.1814
3 0.581 0.1659
---- t3 -----
0 0.5045 0.0966
1 0.6738 0.1705
2 0.6405 0.1991
3 0.5904 0.1799
---- t2 -----
0 0.5029 0.0963
1 0.6768 0.17
2 0.6513 0.2053
3 0.5958 0.182
---- t1 -----
0 0.5024 0.0962
1 0.6891 0.1742
2 0.6718 0.2258
3 0.6104 0.2025
---- t -----
0 0.5017 0.0961
1 0.6976 0.1755
2 0.6829 0.2321
3 0.6201 0.2075

delta_collect_timestamp_t-t1     4.235348
delta_collect_timestamp_t1-t2    3.413571
delta_collect_timestamp_t2-t3    3.116624
delta_collect_timestamp_t3-t4    3.233622
